# Supplementary material for: Decentralized Gaussian Mixture Fusion through Unified Quotient Approximations
Source: arXiv:1907.04008 source file (2019-07-09)
Supplement: Supplementary file 1 [file appendix.tex]

The gradient vector and Hessian matrix for the function $f(x_k) = -\log \tilde{m}_{qr}(x_k)$ are provided for both exact and WEP GM DDF. In general, 
\begin{align*}
f(x_k) = -\log \tilde{m}_{qr}(x_k) = -\log {\cal N}(\mu_t, \Sigma_t) + \log u(x_k), %\nonumber %\label{eq:logmtilde}
\end{align*}
where we have for exact DDF
\begin{align*}
u(x_k) = \sum_{c=1}^{M_c}{w_c  {\cal N}(\mu_c, \Sigma_c)},
\end{align*}
and for WEP DDF
\begin{align*}
u(x_k) &= [p_i(x_k)]^{1-\omega}[p_j(x_k)]^{\omega} \nonumber \\
&= \bigsquare{ \sum_{h=1}^{M_h}{w_h  {\cal N}(\mu_h, \Sigma_h)}}^{1-\omega} \bigsquare{\sum_{l=1}^{M_l}{w_l  {\cal N}(\mu_l, \Sigma_l)} }^{\omega}.
\end{align*}
The following definitions will be useful. If $x_k \in \mathbb{R}^d$ for the GM pdf $p_{v}(x_k) = \sum_{a=1}^{M_a}{w_a {\cal N}(\mu_a, \Sigma_a)}$, define the functions ${\bf i}_a(x_k) =  \Sigma^{-1}_a [\mu_a - x_k]$ and 
\begin{align}
r_v(x_k) = \frac{ \sum_{a=1}^{M_a}{w_a {\cal N}(\mu_a, \Sigma_a) {\bf i}_a(x_k)} }{ p_{v}(x_k) }.
\end{align}
The derivative of $r_v(x_k)$ is the $d \times d$ matrix function
\begin{align}
h_v(x_k) = &\frac{ \sum_{a=1}^{M_a}{w_a {\cal N}(\mu_a, \Sigma_a) \bigcurly{ {\bf i}_a(x_k){\bf i}^T_a(x_k) - \Sigma^{-1}_a }} }{ p_{v}(x_k) } \nonumber \\
&- r_v(x_k) r^T_v(x_k). 
\end{align}
For exact DDF, the gradient $\nabla f(x_k)$ and Hessian  ${\cal H}(x_k)$ are
\begin{align}
\nabla f(x_k) &= -{\bf i}_t(x_k) + r_c(x_k), \\
{\cal H}(x_k) &= \Sigma^{-1}_t + h_t(x_k).
\end{align}
For WEP DDF, we obtain
\begin{align}
\nabla f(x_k) &= -{\bf i}_t(x_k) + (1-\omega) \cdot r_i(x_k) + \omega \cdot r_j(x_k), \\
{\cal H}(x_k) &= \Sigma^{-1}_t + (1-\omega) \cdot h_i(x_k) + \omega \cdot h_j(x_k).
\end{align}
